# Supplementary material for: PitVis-2023 Challenge: Workflow Recognition in videos of Endoscopic Pituitary Surgery
Source: arXiv:2409.01184 ancillary file (2024-09-02)
Supplement: Supplementary file 1 [file BIAS-reporting-guideline.pdf]

# Appendix A: BIAS Reporting Guideline

| Section/<br>Topic                         | Parameter name                     | Item<br>No | Checklist Item                                                                                                                                                                                                                                                                                                                                                                                                                                                                                                                                                                                                                                            | Reported on<br>page No |
|-------------------------------------------|------------------------------------|------------|-----------------------------------------------------------------------------------------------------------------------------------------------------------------------------------------------------------------------------------------------------------------------------------------------------------------------------------------------------------------------------------------------------------------------------------------------------------------------------------------------------------------------------------------------------------------------------------------------------------------------------------------------------------|------------------------|
| TITLE,<br>ABSTRACT,<br>KEYWORDS           | Title                              | 1          | Use the title to convey the essential information on the <b>challenge mission</b> .<br><br>The title should ... <ul style="list-style-type: none"> <li>... identify the paper as biomedical image analysis challenge.</li> <li>... indicate the image modality(ies) applied with a commonly used term in the title.</li> <li>... indicate the task and/or task category (e.g. classification, segmentation; see parameter 18) with a commonly used term in the title.</li> <li>... (optionally) include information on the biomedical target application.</li> <li>... (optionally) include the year for repeated challenges with fixed cycle.</li> </ul> | 1                      |
|                                           | Abstract                           | 2          | Provide a <b>summary</b> of the challenge purpose, design and results and report the main conclusion(s).                                                                                                                                                                                                                                                                                                                                                                                                                                                                                                                                                  | 1                      |
|                                           | Keywords                           | 3          | List the primary <b>keywords</b> that characterize the challenge.                                                                                                                                                                                                                                                                                                                                                                                                                                                                                                                                                                                         | 1                      |
|                                           |                                    |            |                                                                                                                                                                                                                                                                                                                                                                                                                                                                                                                                                                                                                                                           |                        |
| INTRO-<br>DUCTION                         | Challenge motivation and objective | 4a         | Provide a general introduction to the topic from a <b>biomedical point of view</b> . This should include the envisioned biomedical impact (short-term and/or long-term).                                                                                                                                                                                                                                                                                                                                                                                                                                                                                  | 2                      |
|                                           |                                    | 4b         | Provide a general introduction to the topic from a <b>technical point of view</b> . This should include an overview of the state of the art along the envisioned technical/methodological impact.                                                                                                                                                                                                                                                                                                                                                                                                                                                         | 2                      |
|                                           |                                    | 4c         | Based on the biomedical and technical motivation, provide a concise statement of the <b>primary challenge objective</b> . This should include a <b>statement of the task</b> .                                                                                                                                                                                                                                                                                                                                                                                                                                                                            | 2                      |
| METHODS<br>Challenge<br>organi-<br>zation | Challenge name                     | 5a         | Provide a <b>representative name</b> of the challenge.<br><i>Example: MICCAI Endoscopic Vision Challenge 2015</i>                                                                                                                                                                                                                                                                                                                                                                                                                                                                                                                                         | 2                      |
|                                           |                                    | 5b         | Provide the <b>acronym</b> of the challenge (if any).<br><i>Example: EndoVis15</i>                                                                                                                                                                                                                                                                                                                                                                                                                                                                                                                                                                        | 2                      |
|                                           | Organizing team                    | 6          | Provide information on the <b>organizing team</b> (names and affiliations).                                                                                                                                                                                                                                                                                                                                                                                                                                                                                                                                                                               | 1,6,20                 |
|                                           | Life cycle type                    | 7          | Define the intended <b>submission cycle</b> of the challenge. Include information on whether/how the challenge has been/will be continued after the present study.<br><i>Examples:</i> <ul style="list-style-type: none"> <li>One-time event with fixed submission deadline</li> </ul>                                                                                                                                                                                                                                                                                                                                                                    | 6                      |

|                                     |            |                                                                                                                                                                                                                                                                                                                                                                                                                                                        |     |
|-------------------------------------|------------|--------------------------------------------------------------------------------------------------------------------------------------------------------------------------------------------------------------------------------------------------------------------------------------------------------------------------------------------------------------------------------------------------------------------------------------------------------|-----|
|                                     |            | <ul style="list-style-type: none"> <li>• Open call</li> <li>• Repeated event with annual fixed submission deadline</li> </ul>                                                                                                                                                                                                                                                                                                                          |     |
| <b>Challenge venue and platform</b> | <b>8a</b>  | Report the <b>event</b> (e.g. conference) that was <b>associated</b> with the challenge (if any).                                                                                                                                                                                                                                                                                                                                                      | 2,6 |
|                                     | <b>8b</b>  | Report the <b>platform</b> (e.g. grand-challenge.org) used to run the challenge.                                                                                                                                                                                                                                                                                                                                                                       | 6   |
|                                     | <b>8c</b>  | Provide the <b>URL</b> for the challenge website (if any).                                                                                                                                                                                                                                                                                                                                                                                             | 6   |
| <b>Participation policies</b>       | <b>9a</b>  | Define the <b>allowed user interaction</b> of the algorithms assessed (e.g. only (semi-) automatic methods allowed).                                                                                                                                                                                                                                                                                                                                   | 6   |
|                                     | <b>9b</b>  | Define the policy on the <b>usage of training data</b> . The data used to train algorithms may, for example, have been restricted to the data provided by the challenge or to publicly available data including (open) pre-trained nets.                                                                                                                                                                                                               | 6   |
|                                     | <b>9c</b>  | Define the <b>participation policy for members of the organizers' institutes</b> . For example, members of the organizers' institutes could participate in the challenge but were not eligible for awards.                                                                                                                                                                                                                                             | 6   |
|                                     | <b>9d</b>  | Define the <b>award policy</b> . In particular, provide details with respect to challenge prizes.                                                                                                                                                                                                                                                                                                                                                      | 6   |
|                                     | <b>9e</b>  | Define the policy for <b>results announcement</b> .<br><i>Examples:</i> <ul style="list-style-type: none"> <li>• Top three performing methods were announced publicly.</li> <li>• Participating teams could choose whether the performance results will be made public.</li> </ul>                                                                                                                                                                     | 6   |
|                                     | <b>9f</b>  | Define the <b>publication policy</b> . In particular, provide details on ... <ul style="list-style-type: none"> <li>• ... who of the participating teams/the participating teams' members qualified as author</li> <li>• ... whether the participating teams could publish their own results separately, and (if so)</li> <li>• ... whether an embargo time was defined (so that challenge organizers can publish a challenge paper first).</li> </ul> | 20  |
| <b>Submission method</b>            | <b>10a</b> | Describe the method used for result submission. If available, provide a link to the <b>submission instructions</b> .<br><i>Examples:</i> <ul style="list-style-type: none"> <li>• Docker container on the Synapse platform. Link to submission instructions: &lt;URL&gt;</li> <li>• Algorithm output was sent to organizers via e-mail. Submission instructions were sent by e-mail.</li> </ul>                                                        | 6   |
|                                     | <b>10b</b> | Provide information on the possibility for participating teams to <b>evaluate</b> their <b>algorithms before submitting</b> final results. For example, many                                                                                                                                                                                                                                                                                           | 6   |

challenges allow submission of multiple results, and only the last run is officially counted to compute challenge results.

|                                                   |                                             |                                                                                                                                                                                                                                                                                                                                                                                                                                                                                                                                          |             |
|---------------------------------------------------|---------------------------------------------|------------------------------------------------------------------------------------------------------------------------------------------------------------------------------------------------------------------------------------------------------------------------------------------------------------------------------------------------------------------------------------------------------------------------------------------------------------------------------------------------------------------------------------------|-------------|
| <b>Challenge schedule</b>                         | <b>11</b>                                   | Provide a <b>timetable</b> for the challenge. Preferably, this should include <ul style="list-style-type: none"> <li>the release date(s) of the training cases (if any)</li> <li>the registration date/period</li> <li>the release date(s) of the test cases and validation cases (if any)</li> <li>the submission date(s)</li> <li>associated workshop days (if any)</li> <li>the release date(s) of the results</li> </ul>                                                                                                             | <b>6</b>    |
|                                                   | <b>12</b>                                   | Indicate whether <b>ethics approval</b> was necessary for the data. If yes, provide details on the ethics approval, preferably institutional review board, location, date and number of the ethics approval (if applicable). Add the URL or a <b>reference to the document</b> of the ethics approval (if available).                                                                                                                                                                                                                    | <b>6</b>    |
| <b>Data usage agreement</b>                       | <b>13</b>                                   | Clarify how the data can be used and distributed by the teams that participate in the challenge and by others. This should include the explicit <b>listing of the license</b> applied.<br><i>Examples:</i> <ul style="list-style-type: none"> <li>CC BY (Attribution)</li> <li>CC BY-SA (Attribution-ShareAlike)</li> <li>CC BY-ND (Attribution-NoDerivs)</li> <li>CC BY-NC (Attribution-NonCommercial)</li> <li>CC BY-NC-SA (Attribution-NonCommercial-ShareAlike)</li> <li>CC BY-NC-ND (Attribution-NonCommercial-NoDerivs)</li> </ul> | <b>20</b>   |
| <b>Code availability</b>                          | <b>14a</b>                                  | Provide information on the <b>accessibility of the organizers' evaluation software</b> (e.g. code to produce rankings). Preferably, provide a link to the code and add information on the supported platforms.                                                                                                                                                                                                                                                                                                                           | <b>6</b>    |
|                                                   | <b>14b</b>                                  | In an analogous manner, provide information on the <b>accessibility of the participating teams' code</b> .                                                                                                                                                                                                                                                                                                                                                                                                                               | <b>6</b>    |
| <b>Conflicts of interest</b>                      | <b>15</b>                                   | Provide information related to conflicts of interest. In particular provide information related to <b>sponsoring/funding</b> of the challenge. Also, state explicitly who had <b>access to the test case labels</b> and when.                                                                                                                                                                                                                                                                                                            | <b>6,20</b> |
| <b>Author contributions</b>                       | <b>16</b>                                   | List the <b>contributions</b> of all authors to the paper (preferably in the appendix).                                                                                                                                                                                                                                                                                                                                                                                                                                                  | <b>20</b>   |
| <b>METHODS</b><br><b>Mission of the challenge</b> | <b>Field(s) of application</b><br><b>17</b> | State the <b>main field(s) of application</b> that the participating algorithms target.<br><i>Examples:</i> <ul style="list-style-type: none"> <li>Diagnosis</li> <li>Education</li> <li>Intervention assistance</li> </ul>                                                                                                                                                                                                                                                                                                              | <b>2,4</b>  |

|                              |            |                                                                                                                                                                                                                                                                                                                                                                                                                                                                                                                                                                                |            |
|------------------------------|------------|--------------------------------------------------------------------------------------------------------------------------------------------------------------------------------------------------------------------------------------------------------------------------------------------------------------------------------------------------------------------------------------------------------------------------------------------------------------------------------------------------------------------------------------------------------------------------------|------------|
|                              |            | <ul style="list-style-type: none"> <li>• Intervention follow-up</li> <li>• Intervention planning</li> <li>• Prognosis</li> <li>• Research</li> <li>• Screening</li> <li>• Training</li> <li>• Cross-phase</li> </ul>                                                                                                                                                                                                                                                                                                                                                           |            |
| <b>Task category(ies)</b>    | <b>18</b>  | State the <b>task category(ies)</b> .<br><i>Examples:</i> <ul style="list-style-type: none"> <li>• Classification</li> <li>• Detection</li> <li>• Localization</li> <li>• Modeling</li> <li>• Prediction</li> <li>• Reconstruction</li> <li>• Registration</li> <li>• Retrieval</li> <li>• Segmentation</li> <li>• Tracking</li> </ul>                                                                                                                                                                                                                                         | <b>3,4</b> |
| <b>Cohorts</b>               |            | We distinguish between the <i>target cohort</i> and the <i>challenge cohort</i> . For example, a challenge could be designed around the task of medical instrument tracking in robotic kidney surgery. While the challenge could be based on ex vivo data obtained from a laparoscopic training environment with porcine organs (challenge cohort), the final biomedical application (i.e. robotic kidney surgery) would be targeted on real patients with certain characteristics defined by inclusion criteria such as restrictions regarding gender or age (target cohort). |            |
|                              | <b>19a</b> | Describe the <b>target cohort</b> , i.e. the subjects/objects from whom/which the data would be acquired in the final biomedical application.                                                                                                                                                                                                                                                                                                                                                                                                                                  | <b>8</b>   |
|                              | <b>19b</b> | Describe the <b>challenge cohort</b> , i.e. the subject(s)/object(s) from whom/which the challenge data was acquired.                                                                                                                                                                                                                                                                                                                                                                                                                                                          | <b>8</b>   |
| <b>Imaging modality(ies)</b> | <b>20</b>  | Specify the <b>imaging technique(s)</b> applied in the challenge.                                                                                                                                                                                                                                                                                                                                                                                                                                                                                                              | <b>8</b>   |
| <b>Context information</b>   |            | Provide additional <b>information given along with the images</b> . The information may correspond ...                                                                                                                                                                                                                                                                                                                                                                                                                                                                         |            |
|                              | <b>21a</b> | ... directly to the <b>image data</b> (e.g. tumor volume). If necessary, differentiate between target and challenge cohort.                                                                                                                                                                                                                                                                                                                                                                                                                                                    | <b>8</b>   |
|                              | <b>21b</b> | ... to the <b>patient</b> in general (e.g. gender, medical history). If necessary, differentiate between target and challenge cohort.                                                                                                                                                                                                                                                                                                                                                                                                                                          | <b>8</b>   |
|                              | <b>21c</b> | ... to the <b>acquisition process</b> (e.g. medical device data during endoscopic surgery, calibration data for an image modality). If necessary, differentiate between target and challenge cohort.                                                                                                                                                                                                                                                                                                                                                                           | <b>8</b>   |
| <b>Target entity(ies)</b>    | <b>22a</b> | Describe the <b>data origin</b> , i.e. the region(s)/part(s) of subject(s)/object(s) from whom/which the image data would be acquired in the final                                                                                                                                                                                                                                                                                                                                                                                                                             | <b>8</b>   |

biomedical application (e.g. brain shown in computed tomography (CT) data, abdomen shown in laparoscopic video data, operating room shown in video data, thorax shown in fluoroscopy video). If necessary, differentiate between target and challenge cohort.

|            |                                                                                                                                                                                                                                                                                                                                                         |     |
|------------|---------------------------------------------------------------------------------------------------------------------------------------------------------------------------------------------------------------------------------------------------------------------------------------------------------------------------------------------------------|-----|
| <b>22b</b> | Describe the <b>algorithm target</b> , i.e. the structure(s)/subject(s)/object(s)/component(s) that the participating algorithms have been designed to focus on (e.g. tumor in the brain, tip of a medical instrument, nurse in an operating theater, catheter in a fluoroscopy scan). If necessary, differentiate between target and challenge cohort. | 4,8 |
|------------|---------------------------------------------------------------------------------------------------------------------------------------------------------------------------------------------------------------------------------------------------------------------------------------------------------------------------------------------------------|-----|

|                          |           |                                                                                                                                                                                                                                                                                                                                                                                                                                                                                                                                                                                                                                                                                                                                                                                                                                                         |   |
|--------------------------|-----------|---------------------------------------------------------------------------------------------------------------------------------------------------------------------------------------------------------------------------------------------------------------------------------------------------------------------------------------------------------------------------------------------------------------------------------------------------------------------------------------------------------------------------------------------------------------------------------------------------------------------------------------------------------------------------------------------------------------------------------------------------------------------------------------------------------------------------------------------------------|---|
| <b>Assessment aim(s)</b> | <b>23</b> | Identify the <b>property(ies) of the algorithms to be optimized</b> to perform well in the challenge. If multiple properties were assessed, prioritize them (if appropriate). The properties should then be reflected in the metrics applied (parameter 29), and the priorities should be reflected in the ranking when combining multiple metrics that assess different properties. <ul style="list-style-type: none"> <li>• <i>Example 1:</i> Find liver segmentation algorithm for CT images that processes CT images of a certain size in less than a minute on a certain hardware with an error that reflects inter-rater variability of experts.</li> <li>• <i>Example 2:</i> Find lung tumor detection algorithm with high sensitivity and specificity for mammography images.</li> </ul> Corresponding metrics are listed below (parameter 29). | 7 |
|--------------------------|-----------|---------------------------------------------------------------------------------------------------------------------------------------------------------------------------------------------------------------------------------------------------------------------------------------------------------------------------------------------------------------------------------------------------------------------------------------------------------------------------------------------------------------------------------------------------------------------------------------------------------------------------------------------------------------------------------------------------------------------------------------------------------------------------------------------------------------------------------------------------------|---|

|                                               |                       |            |                                                                                                                                                                                                                                                                                              |      |
|-----------------------------------------------|-----------------------|------------|----------------------------------------------------------------------------------------------------------------------------------------------------------------------------------------------------------------------------------------------------------------------------------------------|------|
| <b>METHODS</b><br><b>Challenge data sets</b>  | <b>Data source(s)</b> | <b>24a</b> | Specify the <b>device(s)</b> used to acquire the challenge data. This includes details on the device(s) used to acquire the imaging data (e.g. manufacturer) as well as information on additional devices used for performance assessment (e.g. tracking system used in a surgical setting). | 8    |
|                                               |                       | <b>24b</b> | Describe relevant details on the imaging process/ <b>data acquisition</b> for each acquisition device (e.g. image acquisition protocol(s)).                                                                                                                                                  | 8    |
|                                               |                       | <b>24c</b> | Specify the <b>center(s)/institute(s)</b> in which the data was acquired and/or the <b>data providing platform/source</b> (e.g. previous challenge). If this information is not provided (e.g. for anonymization reasons), specify why.                                                      | 8    |
|                                               |                       | <b>24d</b> | Describe relevant <b>characteristics</b> (e.g. level of expertise) <b>of the subjects</b> (e.g. surgeon)/objects (e.g. robot) involved in the data acquisition process (if any).                                                                                                             | 8    |
| <b>Training and test case characteristics</b> |                       | <b>25a</b> | State what is meant by one <b>case</b> in this challenge. A case encompasses all data that is processed to produce one result that is then compared to the corresponding reference result (i.e. the desired algorithm output).                                                               | 7,15 |

Examples:

- Training and test cases both represented a CT image of a human brain. Training cases had a weak annotation (tumor present or not and tumor volume (if any)) while the test cases were annotated with the tumor contour (if any).
- A case refers to all information that is available for one particular patient in a specific study. This information always includes the image information as specified in *data source(s)* (parameter 24) and may include context information (parameter 21). Both training and test cases were annotated with survival (binary) 5 years after (first) image was taken.

|                                      |            |                                                                                                                                                                                                                                                                                                                                                                                                                                    |   |
|--------------------------------------|------------|------------------------------------------------------------------------------------------------------------------------------------------------------------------------------------------------------------------------------------------------------------------------------------------------------------------------------------------------------------------------------------------------------------------------------------|---|
|                                      | <b>25b</b> | State the <b>total number</b> of cases as well as the number of training, validation and test cases separately.                                                                                                                                                                                                                                                                                                                    | 8 |
|                                      | <b>25c</b> | Explain <b>why a total number</b> of cases and <b>the specific proportion</b> of training, validation and test cases was chosen.                                                                                                                                                                                                                                                                                                   | 8 |
|                                      | <b>25d</b> | Mention <b>further important characteristics</b> of the training, validation and test cases (e.g. class distribution in classification tasks chosen according to real-world distribution vs. equal class distribution) and justify the choice.                                                                                                                                                                                     | 9 |
| <b>Annotation characteristics</b>    | <b>26a</b> | Describe the <b>method for determining the reference annotation</b> , i.e. the desired algorithm output. Provide the information separately for the training, validation and test cases if necessary. Possible methods include <i>manual image annotation</i> , <i>in silico ground truth generation</i> and <i>annotation by automatic methods</i> .<br>If human annotation was involved, state the <b>number of annotators</b> . | 8 |
|                                      | <b>26b</b> | Provide the <b>instructions given to the annotators</b> (if any) prior to the annotation. This may include description of a training phase with the software. Provide the information separately for the training, validation and test cases if necessary. Preferably, provide a link to the <b>annotation protocol</b> .                                                                                                          | 8 |
|                                      | <b>26c</b> | Provide <b>details on the subject(s)/algorithm(s) that annotated</b> the cases (e.g. information on <b>level of expertise</b> such as number of years of professional experience, medically-trained or not). Provide the information separately for the training, validation and test cases if necessary.                                                                                                                          | 8 |
|                                      | <b>26d</b> | Describe the <b>method(s) used to merge multiple annotations</b> for one case (if any). Provide the information separately for the training, validation and test cases if necessary.                                                                                                                                                                                                                                               | 8 |
| <b>Data pre-processing method(s)</b> | <b>27</b>  | Describe the <b>method(s) used for pre-processing</b> the raw training data before it is provided to the participating teams. Provide the information separately for the training, validation and test cases if necessary.                                                                                                                                                                                                         | 8 |

|                                                       |                                    |                                                                                               |                                                                                                                                                                                                                                                                                                                                                                                                                                                                                                                                            |       |
|-------------------------------------------------------|------------------------------------|-----------------------------------------------------------------------------------------------|--------------------------------------------------------------------------------------------------------------------------------------------------------------------------------------------------------------------------------------------------------------------------------------------------------------------------------------------------------------------------------------------------------------------------------------------------------------------------------------------------------------------------------------------|-------|
|                                                       | <b>Sources of error</b>            | <b>28a</b>                                                                                    | Describe the most relevant <b>possible error sources related to the image annotation</b> . If possible, <b>estimate the magnitude</b> (range) of these errors, using inter-and intra-annotator variability, for example. Provide the information separately for the training, validation and test cases, if necessary.                                                                                                                                                                                                                     | 8     |
|                                                       |                                    | <b>28b</b>                                                                                    | In an analogous manner, describe and quantify <b>other relevant sources of error</b> .                                                                                                                                                                                                                                                                                                                                                                                                                                                     | 8     |
| <b>METHODS</b><br><b>Assess-<br/>ment<br/>methods</b> | <b>Metric(s)</b>                   | <b>29a</b>                                                                                    | Define the <b>metric(s) to assess a property of an algorithm</b> . These metrics should reflect the desired algorithm properties described in <i>assessment aim(s)</i> (parameter 21). State which metric(s) were used to compute the ranking(s) (if any).<br><ul style="list-style-type: none"><li>• <i>Example 1:</i> Dice Similarity Coefficient (DSC) and run-time</li><li>• <i>Example 2:</i> Area under curve (AUC)</li></ul>                                                                                                        | 7     |
|                                                       |                                    | <b>29b</b>                                                                                    | <b>Justify why</b> the metric(s) was/were chosen, preferably with reference to the biomedical application.                                                                                                                                                                                                                                                                                                                                                                                                                                 | 7     |
|                                                       | <b>Ranking<br/>method(s)</b>       | <b>30a</b>                                                                                    | Describe the <b>method used to compute a performance rank</b> for all submitted algorithms based on the generated metric results on the test cases. Typically the text will describe how results obtained per case and metric are aggregated to arrive at a final score/ranking.                                                                                                                                                                                                                                                           | 15    |
|                                                       |                                    | <b>30b</b>                                                                                    | Describe the method(s) used to manage <b>submissions with missing results</b> on test cases.                                                                                                                                                                                                                                                                                                                                                                                                                                               | 15    |
|                                                       |                                    | <b>30c</b>                                                                                    | <b>Justify why</b> the described ranking scheme(s) was/were used.                                                                                                                                                                                                                                                                                                                                                                                                                                                                          | 15    |
|                                                       | <b>Statistical<br/>analyses</b>    | <b>31a</b>                                                                                    | Provide <b>details for all statistical methods</b> used in the scope of the challenge analysis. This may include<br><ul style="list-style-type: none"><li>• description of the <b>missing data handling</b>,</li><li>• details about the assessment of <b>variability of rankings</b>,</li><li>• description of any method used to assess <b>whether the data met the assumptions</b>, required for the particular statistical approach, or</li><li>• indication of any <b>software product</b> that was used for data analysis.</li></ul> | 15    |
|                                                       |                                    | <b>31b</b>                                                                                    | <b>Justify why</b> the described statistical method(s) was/were used.                                                                                                                                                                                                                                                                                                                                                                                                                                                                      | 7,15  |
| <b>RESULTS</b><br><b>Challenge<br/>outcome</b>        | <b>Challenge<br/>submissions</b>   | Provide <b>summarizing information</b> on ...                                                 |                                                                                                                                                                                                                                                                                                                                                                                                                                                                                                                                            |       |
|                                                       |                                    | <b>32a</b>                                                                                    | ... the <b>number of registrations</b> .                                                                                                                                                                                                                                                                                                                                                                                                                                                                                                   | 11    |
|                                                       |                                    | <b>32b</b>                                                                                    | ... the <b>number of participating teams</b> that provided valid submissions (if applicable in each phase).                                                                                                                                                                                                                                                                                                                                                                                                                                | 11    |
|                                                       |                                    | <b>32c</b>                                                                                    | ... the <b>number of participating teams</b> that the <b>paper</b> refers to (with <b>justification</b> ).                                                                                                                                                                                                                                                                                                                                                                                                                                 | 11,20 |
|                                                       | <b>Information on<br/>selected</b> | Provide the following information for the participating teams that are included in the paper: |                                                                                                                                                                                                                                                                                                                                                                                                                                                                                                                                            |       |
|                                                       |                                    | <b>33a</b>                                                                                    | <b>Team identifier</b> .                                                                                                                                                                                                                                                                                                                                                                                                                                                                                                                   | 11    |

|                   |                                        |            |                                                                                                                                                                                                                                                                                                                                  |       |
|-------------------|----------------------------------------|------------|----------------------------------------------------------------------------------------------------------------------------------------------------------------------------------------------------------------------------------------------------------------------------------------------------------------------------------|-------|
|                   | <b>participating teams</b>             | <b>33b</b> | A <b>method description</b> including parameter instantiation and/or a reference/URL to a document containing this information.                                                                                                                                                                                                  | 11-15 |
|                   | <b>Metric values</b>                   | <b>34</b>  | Provide raw and/or <b>aggregated metric values</b> (including measure of variability) for all participating teams and each metric (if applicable) as well as the <b>numbers of test set submissions</b> (the last one was used to compute metric(s)) for each participating team.                                                | 15-18 |
|                   | <b>Ranking(s)</b>                      | <b>35a</b> | Report the <b>ranking(s)</b> (if any) including the number of test set submissions for each participating team.                                                                                                                                                                                                                  | 15-18 |
|                   |                                        | <b>35b</b> | Provide the results of the <b>statistical analyses</b> .                                                                                                                                                                                                                                                                         | 15-18 |
|                   | <b>Further Analyses</b>                | <b>36</b>  | Present results of further analyses (if applicable), e.g. related to <ul style="list-style-type: none"> <li>• <b>combining algorithms</b> via ensembling,</li> <li>• <b>inter-algorithm variability</b>,</li> <li>• <b>common problems/biases</b> of the submitted methods, or</li> <li>• <b>ranking variability</b>.</li> </ul> | 15-18 |
|                   |                                        |            |                                                                                                                                                                                                                                                                                                                                  |       |
| <b>DISCUSSION</b> | <b>Summary</b>                         | <b>37</b>  | Summarize the <b>main results</b> of the challenge.                                                                                                                                                                                                                                                                              | 19    |
|                   | <b>Impact</b>                          | <b>38a</b> | Describe the (expected) <b>biomedical impact</b> of the challenge in the context of the state of the art with reference to the challenge motivation (parameter 4a).                                                                                                                                                              | 19    |
|                   |                                        | <b>38b</b> | Describe the (expected) <b>technical impact</b> of the challenge in the context of the state of the art with reference to the challenge motivation (parameter 4b).                                                                                                                                                               | 19    |
|                   | <b>Discussion of challenge results</b> | <b>39a</b> | Provide a detailed discussion and conclusion whether the <b>task is now solved</b> in a satisfactory way (e.g. the remaining errors are comparable to inter-annotator variability).                                                                                                                                              | 19    |
|                   |                                        | <b>39b</b> | Provide a detailed <b>analysis of individual cases</b> , in which the majority of algorithms performed poorly (if any).                                                                                                                                                                                                          | 16-18 |
|                   |                                        | <b>39c</b> | Provide a <b>discussion on advantages and disadvantages of the submitted methods</b> . Include time and memory consumption comparison if time and memory were not among the metrics.                                                                                                                                             | 15-18 |
|                   | <b>Limitations of the challenge</b>    | <b>40</b>  | Discuss <b>limitations</b> related to the challenge design and execution.                                                                                                                                                                                                                                                        | 19    |
|                   | <b>Future work</b>                     | <b>41</b>  | Provide <b>recommendations for future work</b> and maintenance plans for the challenge and its website (if any).                                                                                                                                                                                                                 | 19    |
|                   | <b>Conclusions</b>                     | <b>42</b>  | Provide a <b>concise conclusion</b> based on the results of the study.                                                                                                                                                                                                                                                           | 19    |
|                   |                                        |            |                                                                                                                                                                                                                                                                                                                                  |       |
